# Supplementary material for: Evaluating the Use of LLMs for Automated DOM-Level Resolution of Web Performance Issues
Source: arXiv:2601.05502 source file (2026-01-09)
Supplement: Supplementary file 1 [file appendix_audit_definitions.tex]

\newpage

\section{Appendix B: Definitions \& Coverage Ratios of Audits}
\label{app:audit_appendix}

\begin{longtable}{l p{2.5cm} p{1.5cm} p{1.5cm} p{1.5cm} p{1.5cm} p{1.5cm}}
    \caption{Comparison of the incidence ratio of audits by category} \\
    \toprule
    \textbf{Category} & \textbf{Audit Name} & \textbf{Original IR} & \textbf{Modified IR} & \textbf{Initial Count} & \textbf{Modified Count} & \textbf{\% Change} \\
    \midrule
    \endfirsthead
    \toprule
    \textbf{Category} & \textbf{Audit Name} & \textbf{Original IR} & \textbf{Modified IR} & \textbf{Initial Count} & \textbf{Modified Count} & \textbf{\% Change} \\
    \midrule
    \endhead
    \midrule
    \multicolumn{7}{r}{{Continued on next page}} \\
    \midrule
    \endfoot
    \bottomrule
    \endlastfoot

    \textbf{SEO \& Accessibility} & & & & & & \\
    & crawlable-anchors & 0.20 & 0.00 & 3 & 0 & -100.00 \\
    & link-text & 0.13 & 0.00 & 2 & 0 & -100.00 \\
    & is-crawlable & 0.13 & 0.00 & 2 & 0 & -100.00 \\
    & meta-description & 0.07 & 0.00 & 1 & 0 & -100.00 \\
    & hreflang & 0.07 & 0.00 & 1 & 0 & -100.00 \\
    & aria-prohibited-attr & 0.07 & 0.00 & 1 & 0 & -100.00 \\
    & aria-hidden-focus & 0.20 & 0.00 & 3 & 0 & -100.00 \\
    & image-alt & 0.13 & 0.00 & 2 & 0 & -100.00 \\
    & aria-allowed-attr & 0.07 & 0.00 & 1 & 0 & -100.00 \\
    & listitem & 0.07 & 0.00 & 1 & 0 & -100.00 \\
    & list & 0.07 & 0.00 & 1 & 0 & -100.00 \\
    & aria-dialog-name & 0.07 & 0.00 & 1 & 0 & -100.00 \\
    & label-content-name-mismatch & 0.07 & 0.00 & 1 & 0 & -100.00 \\
    & input-button-name & 0.07 & 0.00 & 1 & 0 & -100.00 \\
    & html-lang-valid & 0.07 & 0.00 & 1 & 0 & -100.00 \\
    & aria-tooltip-name & 0.07 & 0.00 & 1 & 0 & -100.00 \\
    & link-name & 0.07 & 0.00 & 1 & 0 & -100.00 \\
    \midrule

    \textbf{Network Optimization} & & & & & & \\
    & uses-rel-preconnect & 0.27 & 0.00 & 4 & 0 & -100.00 \\
    & uses-http2 & 0.13 & 0.00 & 2 & 0 & -100.00 \\
    & third-party-cookies & 0.47 & 0.00 & 7 & 0 & -100.00 \\
    & is-on-https & 0.47 & 0.00 & 7 & 0 & -100.00 \\
    & total-byte-weight & 0.33 & 0.07 & 5 & 1 & -80.00 \\
    & uses-text-compression & 0.93 & 0.67 & 14 & 10 & -28.57 \\
    & uses-long-cache-ttl & 0.60 & 0.47 & 9 & 7 & -22.22 \\
    & redirects & 0.07 & 0.07 & 1 & 1 & 0.00 \\
    \midrule

    \textbf{Initial Load Performance} & & & & & & \\
    & charset & 0.20 & 0.00 & 3 & 0 & -100.00 \\
    & lcp-lazy-loaded & 0.13 & 0.00 & 2 & 0 & -100.00 \\
    & offscreen-images & 0.40 & 0.13 & 6 & 2 & -66.67 \\
    & render-blocking-resources & 0.60 & 0.20 & 9 & 3 & -66.67 \\
    & first-contentful-paint & 1.00 & 0.67 & 15 & 10 & -33.33 \\
    & speed-index & 1.00 & 0.80 & 15 & 12 & -20.00 \\
    & largest-contentful-paint-element & 0.93 & 0.87 & 14 & 13 & -7.14 \\
    & prioritize-lcp-image & 0.07 & 0.07 & 1 & 1 & 0.00 \\
    & largest-contentful-paint & 0.93 & 1.67 & 14 & 25 & 78.57 \\
    \midrule

    \textbf{Visual Stability} & & & & & & \\
    & viewport & 0.27 & 0.00 & 4 & 0 & -100.00 \\
    & meta-viewport & 0.20 & 0.00 & 3 & 0 & -100.00 \\
    & image-size-responsive & 0.13 & 0.00 & 2 & 0 & -100.00 \\
    & image-aspect-ratio & 0.13 & 0.00 & 2 & 0 & -100.00 \\
    & font-size & 0.33 & 0.00 & 5 & 0 & -100.00 \\
    & color-contrast & 0.33 & 0.00 & 5 & 0 & -100.00 \\
    & target-size & 0.40 & 0.00 & 6 & 0 & -100.00 \\
    & dom-size & 0.47 & 0.13 & 7 & 2 & -71.43 \\
    & unsized-images & 0.40 & 0.13 & 6 & 2 & -66.67 \\
    & font-display & 0.33 & 0.13 & 5 & 2 & -60.00 \\
    & cumulative-layout-shift & 0.40 & 0.27 & 6 & 4 & -33.33 \\
    & layout-shifts & 0.13 & 0.13 & 2 & 2 & 0.00 \\
    \midrule

    \textbf{Runtime Performance} & & & & & & \\
    & valid-source-maps & 0.07 & 0.00 & 1 & 0 & -100.00 \\
    & inspector-issues & 0.67 & 0.00 & 10 & 0 & -100.00 \\
    & errors-in-console & 0.93 & 0.00 & 14 & 0 & -100.00 \\
    & deprecations & 0.47 & 0.00 & 7 & 0 & -100.00 \\
    & bootup-time & 0.73 & 0.40 & 11 & 6 & -45.45 \\
    & mainthread-work-breakdown & 0.80 & 0.47 & 12 & 7 & -41.67 \\
    & third-party-summary & 0.87 & 0.67 & 13 & 10 & -23.08 \\
    & no-document-write & 0.13 & 0.13 & 2 & 2 & 0.00 \\
    \midrule

    \textbf{Resource Optimization} & & & & & & \\
    & duplicated-javascript & 0.07 & 0.00 & 1 & 0 & -100.00 \\
    & modern-image-formats & 0.40 & 0.13 & 6 & 2 & -66.67 \\
    & legacy-javascript & 0.87 & 0.33 & 13 & 5 & -61.54 \\
    & unminified-css & 0.13 & 0.07 & 2 & 1 & -50.00 \\
    & uses-optimized-images & 0.13 & 0.07 & 2 & 1 & -50.00 \\
    & unused-css-rules & 0.73 & 0.40 & 11 & 6 & -45.45 \\
    & uses-responsive-images & 0.47 & 0.33 & 7 & 5 & -28.57 \\
    & unused-javascript & 1.00 & 0.93 & 15 & 14 & -6.67 \\
    & unminified-javascript & 0.07 & 0.07 & 1 & 1 & 0.00 \\
    \midrule

    \textbf{Interactivity Performance} & & & & & & \\
    & uses-passive-event-listeners & 0.33 & 0.20 & 5 & 3 & -40.00 \\
    & total-blocking-time & 1.00 & 0.80 & 15 & 12 & -20.00 \\
    & max-potential-fid & 1.00 & 0.80 & 15 & 12 & -20.00 \\
    & interactive & 1.00 & 0.87 & 15 & 13 & -13.33 \\
    \midrule
\end{longtable}

\begin{longtable}{|p{0.5cm}|p{3cm}|p{3cm}|p{1cm}|p{3cm}|c|}
\caption{Audit data overview} \label{tab:audit_overview} \\

\hline
\textbf{S/N} & \textbf{Audit Name} & \textbf{Audit Description} & \textbf{Count} & \textbf{Websites} & \textbf{Coverage} \\ \hline
\endfirsthead

\hline
\textbf{S/N} & \textbf{Audit Name} & \textbf{Audit Description} & \textbf{Count} & \textbf{Websites} & \textbf{Coverage} \\ \hline
\endhead

\hline
\multicolumn{6}{|r|}{Continued on next page} \\
\hline
\endfoot

\hline
\endlastfoot

1 & first-contentful-paint & First Contentful Paint marks the time at which the first text or image is painted & 15 & airbnb, aliexpress, ebay, facebook, github, linkedin, medium, netflix, pinterest, quora, reddit, twitch, twitter, walmart, youtube & 100.0 \\ \hline
2 & speed-index & Speed Index shows how quickly the contents of a page are visibly populated & 15 & airbnb, aliexpress, ebay, facebook, github, linkedin, medium, netflix, pinterest, quora, reddit, twitch, twitter, walmart, youtube & 100.0 \\ \hline
3 & total-blocking-time & Sum of all time periods between FCP and Time to Interactive, when task length exceeded 50ms, expressed in milliseconds & 15 & airbnb, aliexpress, ebay, facebook, github, linkedin, medium, netflix, pinterest, quora, reddit, twitch, twitter, walmart, youtube & 100.0 \\ \hline
4 & max-potential-fid & The maximum potential First Input Delay that your users could experience is the duration of the longest task & 15 & airbnb, aliexpress, ebay, facebook, github, linkedin, medium, netflix, pinterest, quora, reddit, twitch, twitter, walmart, youtube & 100.0 \\ \hline
5 & interactive & Time to Interactive is the amount of time it takes for the page to become fully interactive & 15 & airbnb, aliexpress, ebay, facebook, github, linkedin, medium, netflix, pinterest, quora, reddit, twitch, twitter, walmart, youtube & 100.0 \\ \hline
6 & unused-javascript & Reduce unused JavaScript and defer loading scripts until they are required to decrease bytes consumed by network activity & 15 & airbnb, aliexpress, ebay, facebook, github, linkedin, medium, netflix, pinterest, quora, reddit, twitch, twitter, walmart, youtube & 100.0 \\ \hline
7 & largest-contentful-paint-element & This is the largest contentful element painted within the viewport & 14 & airbnb, aliexpress, ebay, facebook, github, linkedin, netflix, pinterest, quora, reddit, twitch, twitter, walmart, youtube & 93.33 \\ \hline
8 & largest-contentful-paint & Largest Contentful Paint marks the time at which the largest text or image is painted & 14 & airbnb, aliexpress, ebay, facebook, github, linkedin, netflix, pinterest, quora, reddit, twitch, twitter, walmart, youtube & 93.33 \\ \hline
9 & errors-in-console & Errors logged to the console indicate unresolved problems & 14 & airbnb, aliexpress, ebay, facebook, github, linkedin, medium, pinterest, quora, reddit, twitch, twitter, walmart, youtube & 93.33 \\ \hline
10 & uses-text-compression & Text-based resources should be served with compression (gzip, deflate or brotli) to minimize total network bytes & 14 & airbnb, aliexpress, ebay, facebook, github, linkedin, medium, netflix, pinterest, quora, reddit, twitch, walmart, youtube & 93.33 \\ \hline
11 & legacy-javascript & Polyfills and transforms enable legacy browsers to use new JavaScript features & 13 & airbnb, aliexpress, ebay, facebook, linkedin, medium, netflix, pinterest, quora, twitch, twitter, walmart, youtube & 86.67 \\ \hline
12 & third-party-summary & Third-party code can significantly impact load performance & 13 & airbnb, aliexpress, ebay, github, linkedin, medium, netflix, pinterest, quora, reddit, twitch, walmart, youtube & 86.67 \\ \hline
13 & mainthread-work-breakdown & Consider reducing the time spent parsing, compiling and executing JS & 12 & airbnb, aliexpress, ebay, github, linkedin, medium, netflix, pinterest, reddit, twitch, walmart, youtube & 80.0 \\ \hline
14 & bootup-time & Consider reducing the time spent parsing, compiling, and executing JS & 11 & aliexpress, ebay, github, linkedin, medium, netflix, pinterest, reddit, twitch, walmart, youtube & 73.33 \\ \hline
15 & unused-css-rules & Reduce unused rules from stylesheets and defer CSS not used for above-the-fold content to decrease bytes consumed by network activity & 11 & airbnb, aliexpress, ebay, github, linkedin, netflix, pinterest, quora, reddit, walmart, youtube & 73.33 \\ \hline
16 & inspector-issues & Issues logged to the `Issues` panel in Chrome Devtools indicate unresolved problems & 10 & airbnb, aliexpress, ebay, linkedin, medium, netflix, twitch, twitter, walmart, youtube & 66.67 \\ \hline
17 & render-blocking-resources & Resources are blocking the first paint of your page & 9 & airbnb, ebay, facebook, github, linkedin, medium, netflix, reddit, youtube & 60.0 \\ \hline
18 & uses-long-cache-ttl & A long cache lifetime can speed up repeat visits to your page & 9 & aliexpress, ebay, linkedin, medium, netflix, pinterest, reddit, twitch, walmart & 60.0 \\ \hline
19 & third-party-cookies & Support for third-party cookies will be removed in a future version of Chrome & 7 & aliexpress, ebay, linkedin, medium, twitch, twitter, walmart & 46.67 \\ \hline
20 & deprecations & Deprecated APIs will eventually be removed from the browser & 7 & aliexpress, ebay, facebook, pinterest, twitch, walmart, youtube & 46.67 \\ \hline
21 & uses-responsive-images & Serve images that are appropriately-sized to save cellular data and improve load time & 7 & aliexpress, ebay, github, pinterest, reddit, twitch, walmart & 46.67 \\ \hline
22 & dom-size & A large DOM will increase memory usage, cause longer [style calculations](https://developers & 7 & airbnb, aliexpress, ebay, github, pinterest, reddit, youtube & 46.67 \\ \hline
23 & is-on-https & All sites should be protected with HTTPS, even ones that don't handle sensitive data & 7 & aliexpress, ebay, linkedin, medium, quora, walmart, youtube & 46.67 \\ \hline
24 & target-size & Touch targets with sufficient size and spacing help users who may have difficulty targeting small controls to activate the targets & 6 & ebay, facebook, github, pinterest, reddit, twitter & 40.0 \\ \hline
25 & modern-image-formats & Image formats like WebP and AVIF often provide better compression than PNG or JPEG, which means faster downloads and less data consumption & 6 & ebay, github, linkedin, pinterest, reddit, twitch & 40.0 \\ \hline
26 & offscreen-images & Consider lazy-loading offscreen and hidden images after all critical resources have finished loading to lower time to interactive & 6 & aliexpress, ebay, github, linkedin, netflix, pinterest & 40.0 \\ \hline
27 & unsized-images & Set an explicit width and height on image elements to reduce layout shifts and improve CLS & 6 & aliexpress, ebay, facebook, github, quora, twitch & 40.0 \\ \hline
28 & cumulative-layout-shift & Cumulative Layout Shift measures the movement of visible elements within the viewport & 6 & aliexpress, ebay, github, pinterest, twitch, walmart & 40.0 \\ \hline
29 & color-contrast & Low-contrast text is difficult or impossible for many users to read & 5 & aliexpress, ebay, facebook, medium, twitter & 33.33 \\ \hline
30 & font-display & Leverage the `font-display` CSS feature to ensure text is user-visible while webfonts are loading & 5 & netflix, pinterest, reddit, twitch, twitter & 33.33 \\ \hline
31 & font-size & Font sizes less than 12px are too small to be legible and require mobile visitors to “pinch to zoom” in order to read & 5 & facebook, netflix, quora, twitch, youtube & 33.33 \\ \hline
32 & uses-passive-event-listeners & Consider marking your touch and wheel event listeners as `passive` to improve your page's scroll performance & 5 & linkedin, pinterest, reddit, twitch, youtube & 33.33 \\ \hline
33 & total-byte-weight & Large network payloads cost users real money and are highly correlated with long load times & 5 & aliexpress, ebay, github, pinterest, youtube & 33.33 \\ \hline
\end{longtable}
